# Supplementary material for: Indexability is Not Enough for Whittle: Improved, Near-Optimal Algorithms for Restless Bandits
Source: arXiv:2211.00112 source file (2023-02-28)
Supplement: Supplementary file 1 [file appendix-10-16-22.tex]

\section{Randomized Action by Sampling and Better Error Bounds}
As discussed in Section~\ref{sec:mf:rounding}, the mean-field action $\malpha$ may not be integral, i.e., $\malpha_{t,i,s}^a$ may be fractional for some $t$, $i$, $s$, and $a$. We described and analyzed the rounding scheme that always satisfied the budget constraint. If one is allowed to satisfy the budget constraint in expectation but violate it by at most $K|S||A|$, which is not a function of $N$ and may be very small compared to the budget, then we can use the randomized unbiased sampling method described below. By using the sampling method we can improve our error bound to (TODO: write the exact bound), analyzed in the appendix.

In the sampling method, first, we deterministically assign $\lfloor \malpha_{t,i,s}^a \rfloor$ arms in $\rmu_{t,i,s}$ to action $a$. Then, we accumulate the remaining fractions $\sum_{a} (\malpha_{t,i,s}^a - \lfloor \malpha_{t,i,s}^a \rfloor)$---we should have an equal number of remaining arms in $\rmu_{t,i,s}$---and assign these remaining arms randomly such that action $a$ gets an arm with probability $\malpha_{t,i,s}^a - \lfloor \malpha_{t,i,s}^a \rfloor$ and no arm with the remaining probability of $1-(\malpha_{t,i,s}^a - \lfloor \malpha_{t,i,s}^a \rfloor)$. This can be done using the bucket sampling approach described below. Notice that the random action we compute using this technique will have the same expected value as the mean-field action, i.e., $\Exp[\ralpha_t] = \malpha_t$ and $\malpha_t$ is an unbiased estimate of $\ralpha_t$.

\paragraph{Bucket Sampling}[TODO: cite. Ask Manish.] Given a vector $x \in [0,1]^n$ such that $\sum_{i \in [n]} x_i = k$, we need to sample a set $\cA$ of exactly $k$ elements from $[n]$ such that $i \in \cA$ with probability $x_i$. We do this as follows: Select $u$ uniformly at random from $[0,1]$. Then, select $\cA$ as
\[
    \cA = \{ i \in [n] \mid (\ell - u) \in [ \sum_{j < i} x_j, \sum_{j \le i} x_j  ) \text{ for some $\ell \in [k]$  }\}.
\]

Let us denote the random $\ralpha_{t,i,s}$ computed from $\malpha_{t,i,s}$ using the bucket sampling approach as $\bucket(\malpha_{t,i,s})$.
%  one-hot representation of the $\cA$ as $\bucket(x) = y \in \{0,1\}^n$ where $y_i = 1$ if $i \in \cA$. Notice that $\bucket(x)$ is random.
 
% In our experiments, both the techniques perform similarly. In the mathematical analysis, the sampling method gives an error proportional to $\sqrt{K}$ while the rounding method gives an error proportional to $K$ given the rewards are similar across arms, i.e., $R_{t,i,s}^a \approx R_{t,j,s}^a$. The formal condition on the reward function and the corresponding bound is given in our analysis in Section~\ref{sec:mf:analysis}.

\begin{proof}
Notice that $\beta_{t,i}$ is an $|S| \times |A|$ right stochastic matrix for every $t$ and $i$. Similarly, $P_{t,i,s}$ is also a right stochastic matrix for every $t,i,s$. Let us define the $|S|\times|S|$ matrix $M_{t,i}$ as $M_{t,i,s,s'} = \sum_{a \in A} \beta_{t,i,s}^a P_{t,i,s,s'}^a$. $M_{t,i}$ is also a right stochastic matrix for every $t$ and $i$ because $\sum_{s'} M_{t,i,s,s'} = \sum_{s'} \sum_{a \in A} \beta_{t,i,s}^a P_{t,i,s,s'}^a = \sum_{a \in A} \beta_{t,i,s}^a \sum_{s'} P_{t,i,s,s'}^a = \sum_{a \in A} \beta_{t,i,s}^a = 1$.

At the initial time-point $t=1$, the real-life state and the mean-field state are both equal to $\mu_1$: $\rmu_1 = \mmu_1 = \mu_1$. At time $t$, there are two sources of divergence (error) between the mean-field state $\mmu_{t}$ and the real-life state $\rmu_{t}$:
\begin{enumerate}
    \item Rounding. For each $t$, we do rounding to compute the real-life action $\ralpha_{t,i,s} = \round(\beta_{t,i,s} \rmu_{t,i,s})$, but not for the mean-field action $\malpha_{t,i,s} = \beta_{t,i,s} \mmu_{t,i,s}$. 
    % Notice that the rounding error may add bias.
    \item Randomness. The real-life state $\rmu_{t+1}$ is a random function of $\ralpha_t$ because of the stochasticity of the transitions.
\end{enumerate}
As mentioned, due to rounding, $\ralpha_{t,i,s}^a$ may not be equal to $\beta_{t,i,s}^a \rmu_{t,i,s}$. Let us define $\rbeta_{t,i,s}^a = \ralpha_{t,i,s}^a / \rmu_{t,i,s}$ if $\rmu_{t,i,s} > 0$ and $\rbeta_{t,i,s}^a = \beta_{t,i,s}^a$ otherwise. As we had defined the right stochastic matrix $M_{t,i}$ based on $\beta_{t,i}$ and $P_{t,i}$, we similarly define the $|S|\times|S|$ right stochastic matrix $\rM_{t,i} = (\sum_a \beta_{t,i,s}^a P_{t,i,s,s'}^a)_{s,s' \in S}$ based on $\rbeta_{t,i}$ and $P_{t,i}$.

Let $(\cF_{t})_{t \in [T]}$ denote the natural filtration with respect to $\rmu_t$, i.e., $\cF_{t}$ models the information available at time $t$. Notice that $\rmu_t$ is $\cF_t$-measurable by definition. 

In the next segment of the proof, we will try to measure how much \textit{new} error is introduced between the mean-field estimate and the real-life process in a given time step due to rounding and randomness. Later in the proof, we shall  quantify how this error gets accumulated over time. 

\textbf{Let us focus on a particular time-step $t \rightarrow (t+1)$.} 
At time $t$, we know the realization of $\rmu_t$. Given $\rmu_t$, we know that $\beta_t$ is deterministic as per its definition. When we use bucket-sampling, the action $\ralpha_{t,i,s} = \bucket(\beta_{t,i,s} \rmu_{t,i,s})$ \textit{partially} random: it is deterministically assigns an action to $\sum_{i,s,a} \lfloor \beta_{t,i,s}^a \rmu_{t,i,s} \rfloor$ arms and randomly to $\sum_{i,s,a} (\beta_{t,i,s}^a \rmu_{t,i,s} - \lfloor \beta_{t,i,s}^a \rmu_{t,i,s} \rfloor) \le K|S||A|$ arms. Notice that the call to the bucket sampling algorithm is made independently for each $i,s$. So, the (at most) $K|S||A|$ arms that are assigned a random action can be partitioned into $K|S|$ groups of size (at most) $|A|$ each, where the action for each of these $K|S|$ groups is picked independently, while the action of the $|A|$ arms within a group may be correlated.

% Remember that $\ralpha_{t,i,s}^a$ is a non-negative integer and denotes the number of arms in cluster $i$ state $s$ at time $t$ for which we play action $a$. Also note that $\sum_{i,s,a} \ralpha_{t,i,s}^a = \sum_{i,s} \rmu_{t,i,s} = N$ for every $t$.

Given $\rmu_{t}$, $\rmu_{t+1}$ is a random variable given by \\
$\rmu_{t+1,i,s'} = \sum_{s, a} \sum_{\ell \in [\ralpha_{t,i,s}^a]} \bI{\{z_{s,\ell}^a = s'\}}$ where $z_{s,\ell}^a \sim P_{t,i,s}^a$ and $\ralpha_{t,i,s}^a$ is the random action found by bucket sampling. 
% If $a$ is random, then with slight abuse of notation, let $P_{t,i,s}^a$ denote its expected value $\Exp_{a}[P_{t,i,s}^a]$, which is deterministic. 
To simplify notation, let us index the $N$ arms by $j = 1, 2, \ldots, N$ and denote arm $j$'s state and action at time $t$ by $s_j$ and $a_j$ ($a_j$ can be random). Let $\cN_i = \{j \mid \text{$j$ is in cluster $i$}\}$. Notice that, by definition, exactly $\ralpha_{t,i,s}^a$ arms will have state and action equal to $s$ and $a$, i.e., $\sum_j \bI{\{s_j = s\}} \bI{\{a_j = a\}} = \ralpha_{t,i,s}^a$. 

Let $Z_j$ be the one-hot random variable that denotes the state of arm $j$ at time $t+1$; so, $(\arg\max_{s} Z_{j,s}) \sim P_{t,s_j}^{a_j}$.  
We can rewrite $\rmu_{t+1}$ as $\rmu_{t+1,i} = \sum_{j \in \cN_i} Z_j$. Further, notice that $\Exp[\rmu_{t+1,i} \mid \cF_t]$ is 
\begin{multline*}
    \Exp[\rmu_{t+1,i} \mid \cF_t] = \Exp \left[ \left. \sum_{j \in \cN_j} Z_j \right| \cF_t \right] = \Exp \left[ \left. \sum_{s, a} \ralpha_{t,i,s}^a P_{t,i,s}^a \right| \cF_t \right] \\
    = \sum_{s} \rmu_{t,i,s} \sum_a \beta_{t,i,s}^a P_{t,i,s}^a = M_{t,i}^\intercal \rmu_{t,i} .
\end{multline*}
Let us now focus on the divergence between $\rmu_{t+1,i}$ and  $\Exp[\rmu_{t+1,i} \mid \cF_t] = M_{t,i}^\intercal \rmu_{t,i}$. We shall show that $\rmu_{t+1}$ is close to $M_t^\intercal \rmu_t$ with high probability.

As discussed earlier, for at least $N - K|S||A|$ arms, $Z_j$ for arm $j$ is picked independently of the other arms (given $\rmu_t$). The remaining $K|S||A|$ arms can be partitioned into $K|S|$ groups $(G_{i,s})_{i \in [K], s \in S}$, where each $G_{i,s}$ is of size at most $|A|$, and there may be a correlation in the actions selected for the arms inside a given group, but not across the groups. For an arm $j$ not in any of these $K|S|$ groups, we have
\begin{itemize}
    \item $Z_j$ is independent of $Z_{k}$ for every $k \neq j$,
    \item $Z_j$ satisfies $-1 \le Z_{j,s} \le 1$ for every $s$, and
    \item $\Exp[Z_j \mid \cF_t] = P_{t,i_j,s_j}^{a_j}$, where $i_j$ is the cluster of arm $j$.
\end{itemize}
On the other hand, we can give similar conditions for the aggregate state of arms in a group $G_{i,s}$. We have
\begin{itemize}
    \item $\sum_{j \in G_{i,s}} Z_j$ is independent of $Z_k$ for every $k \notin G_{i,s}$,
    \item $\sum_{j \in G_{i,s}} Z_j$ satisfies $-|A| \le -|G_{i,s}| \le \sum_{j \in G_{i,s}} Z_{j,s'} \le |G_{i,s}| \le |A|$ for every $s'$, and
    \item $\Exp[ \sum_{j \in G_{i,s}} Z_j \mid \cF_t] = \Exp[ \sum_{j \in G_{i,s}} P_{t,i_j,s_j}^{a_j} \mid \cF_t] $ \\
    $ = \sum_{a} (\beta_{t,i,s}^a \rmu_{t,i,s} - \lfloor \beta_{t,i,s}^a \rmu_{t,i,s} \rfloor) P_{t,i,s}^a $.
\end{itemize}

For the $(N - K|S||A|) + K|S|$ independent variables, where the first $N - K|S||A|$ variables correspond to the arms not in $G_{i,s}$ for any $i,s$ and the remaining $K|S|$ are for the variables $\sum_{j \in G_{i,s}} Z_j$ for some $i,s$, let us apply Hoeffding's inequality  (Lemma~\ref{lm:hoeffding})
\begin{multline*}
    \Prob[ \sum_{j = 1}^N Z_{j,s'} - \sum_{i} (M_{t,i}^\intercal \rmu_{t,i})_{s'} \ge \epsilon ] \\
    \le \exp{ \left(- \frac{2\epsilon^2}{(N - K|S||A|)4 + K|S|(4|A|^2)} \right)}.
\end{multline*}
In a similar manner, we also have $\Prob[ \rmu_{t+1} - M_t^\intercal \rmu_t \le -\epsilon ] \le \exp{ \left(- \frac{\epsilon^2}{2N} \right)}$. 



















Combining this with \eqref{eq:lm:stateError:roundBound}
\begin{multline}\label{eq:lm:stateError:boundt1}
    \Prob[ (\rmu_{t+1} - M_t^\intercal \rmu_t) + (M_t^\intercal \rmu_t - M_t^\intercal \rmu_t) \ge q + \epsilon ] \le \exp{ \left(- \frac{\epsilon^2}{2N} \right)} \\
    \implies \Prob[ \rmu_{t+1} - M_t^\intercal \rmu_t \ge q + \epsilon ] \le \exp{ \left(- \frac{\epsilon^2}{2N} \right)}.
\end{multline}
The bound in \eqref{eq:lm:stateError:boundt1} is true for all $t \ge 1$. Now, pick a time $\tau \le t$. If $\rmu_{\tau+1} - M_{\tau}^\intercal \rmu_{\tau} < q + \epsilon$, 
% or equivalently $\rmu_{\tau+1}^\intercal - \rmu_{\tau}^\intercal M_{\tau} < q^\intercal + \epsilon \b1^\intercal$, where $\b1$ is the vector of all ones, 
then multiplying both sides by $\left(\prod_{\ell = \tau+1}^{t} M_{\ell} \right)^\intercal$ we have
\begin{equation}\label{eq:lm:stateError:boundt2}
    \left(\prod_{\ell = \tau+1}^{t} M_{\ell} \right)^\intercal \rmu_{\tau+1} - \left(\prod_{\ell = \tau}^{t} M_{\ell} \right)^\intercal \rmu_{\tau} < \left(\prod_{\ell = \tau+1}^{t} M_{\ell} \right)^\intercal (q + \b1 \epsilon ),
\end{equation}
where $\b1$ is the vector of all ones. Let us denote the matrix $\prod_{\ell = \tau}^{t} M_{\ell}$ as $M_{\tau:t}$. As $M_{\ell}$ is right stochastic for every $\ell$, $M_{\tau:t}$ is also right stochastic. Combining equations \eqref{eq:lm:stateError:boundt1} and \eqref{eq:lm:stateError:boundt2} for $\tau = 1, \ldots, t$ and applying union-bound we get
\begin{multline*}
    \Prob \left[ \sum_{\tau = 1}^{t} (M_{\tau+1:t}^\intercal \rmu_{\tau+1} - M_{\tau:t}^\intercal \rmu_{\tau}) \ge \sum_{\tau = 1}^{t}  M_{\tau+1:t}^\intercal (q + \b1 \epsilon ) \right] \\
    \le t \exp{ \left(- \frac{\epsilon^2}{2N} \right)}.
\end{multline*}
Notice that sum $\sum_{\tau = 1}^{t} (M_{\tau+1:t}^\intercal \rmu_{\tau+1} - M_{\tau:t}^\intercal \rmu_{\tau})$ is telescoping and is equal to $\rmu_{t+1} - M_{1:t}^\intercal \rmu_1$. Notice that $\rmu_1 = \mu_1 = \mmu_1$, and by definition, $M_{1:t}^\intercal \mmu_1 = \mmu_{t+1}$. So, we get 
\begin{equation}\label{eq:lm:stateError:boundt3}
    \Prob \left[ \rmu_{t+1} - \mmu_{t+1} \ge \sum_{\tau = 1}^{t}  M_{\tau+1:t}^\intercal (q + \b1 \epsilon ) \right] \le t \exp{ \left(- \frac{\epsilon^2}{2N} \right)}.
\end{equation}
Let us now try to bound the error term: $\sum_{\tau = 1}^{t}  M_{\tau+1:t}^\intercal (q + \b1 \epsilon )$. As $M_{\tau+1:t}$ is right stochastic, every element of the matrix is $\le 1$, and therefore, $M_{\tau+1:t}^\intercal q \le \sum_{s'} q_{s'} = \sum_{s,a,s'} P_{t,s,s'}^a = |S||A|$ and $M_{\tau+1:t}^\intercal \b1 \epsilon \le \epsilon |S| $. Putting it back to \eqref{eq:lm:stateError:boundt3} we get
\begin{equation}\label{eq:lm:stateError:boundt4}
    \Prob[ \rmu_{t+1} - \mmu_{t+1} \ge t|S|(|A| + \epsilon) ] \le t \exp{ \left(- \frac{\epsilon^2}{2N} \right)},
\end{equation}
for every $1 \le t \le T-1$ and $\epsilon > 0$. Following analogous steps, we get
\begin{equation}\label{eq:lm:stateError:boundt5}
    \Prob[ \rmu_{t+1} - \mmu_{t+1} \le - t|S|(|A| + \epsilon) ] \le t \exp{ \left(- \frac{\epsilon^2}{2N} \right)},
\end{equation}
for every $1 \le t \le T-1$ and $\epsilon > 0$.
\end{proof}




\section{Additional Lemmas}
\begin{lemma}\label{lm:round}
Given a non-negative real vector $x = (x_1, x_2, \ldots, x_n) \in \bR_{\ge 0}^n$ that sums to an integer $m \in \bZ_{\ge 0}$, $\sum_{i \in [n]} x_i = m$, we can convert $x$ to a non-negative integer vector $z = (z_1, z_2, \ldots, z_n)$ such that $z$ also sums to $m$, the $L_1$ distance between $x$ and $z$ is at most $n/2$, and the $L_{\infty}$ distance between $x$ and $z$ is at most $1$, i.e., $\sum_{i \in [n]} z_i = m$, $\sum_{i \in [n]} |x_i - z_i| \le n/2$, and $\max_{i \in [n]} |x_i - z_i| \le 1$.
\end{lemma}
\begin{proof}
TODO: The proof is trivial but long. Complete later, if required. It feels like it should be a well-known result.

W.l.o.g. we can assume that $0 \le x_i \le 1$ for each $i \in [n]$, because: given an $x$, we can set $\overline{x}_i = x_i - \lfloor x_i \rfloor$ for each $i$ and $\overline{m} = m - \sum_i \lfloor x_i \rfloor$, find a solution of this modified problem $(\overline{x}, \overline{m})$, say $\overline{z}$, then use $\overline{z}$ to construct $z$ as $z_i = \overline{z}_i + \lfloor x_i \rfloor$ for each $i$. It is trivial to check that the solution would satisfy the required conditions.

Now, let $I = \{ i \in [n] \mid 0 < x_i < 1 \}$ be the set of indices that have strictly fractional values. Let us assume that $I$ is in sorted order of $x_i$ values, i.e., $x_{i_j} < x_{i_k}$ for $j < k$ and $i_j, i_k \in I$. Iteratively, we (i) decrease $x_{i_1}$ and increase $x_{i_{|I|}}$ by $min(x_{i_1}, 1-x_{i_{|I|}})$; remove $i_1$ or $i_{|I|}$ (or both) from $I$ if $x_{i_1}$ becomes $0$ or $x_{i_{|I|}}$becomes $1$ after the operation, respectively; repeat until $|I| = 0$. In each step, we decrease the size of $I$ by at least $1$, and in the last step, by $2$. So, this algorithm terminates with an integral solution $z$ that sums up to $m$.


\end{proof}
